# Supplementary material for: Three-states model for calculating the $X$-$X$ rovibrational transition intensities in hydroxyl radical
Source: arXiv:2410.12353 ancillary file (2025-01-14)
Supplement: Supplementary file 1 [file Molecular_functions.pdf]

Supplementary material to paper "Three-states model for calculating the  $X$ - $X$  rovibrational transition intensities in hydroxyl radical" by V.G. Ushakov, A.Yu. Ermilov, and E.S. Medvedev.

### Molecular functions

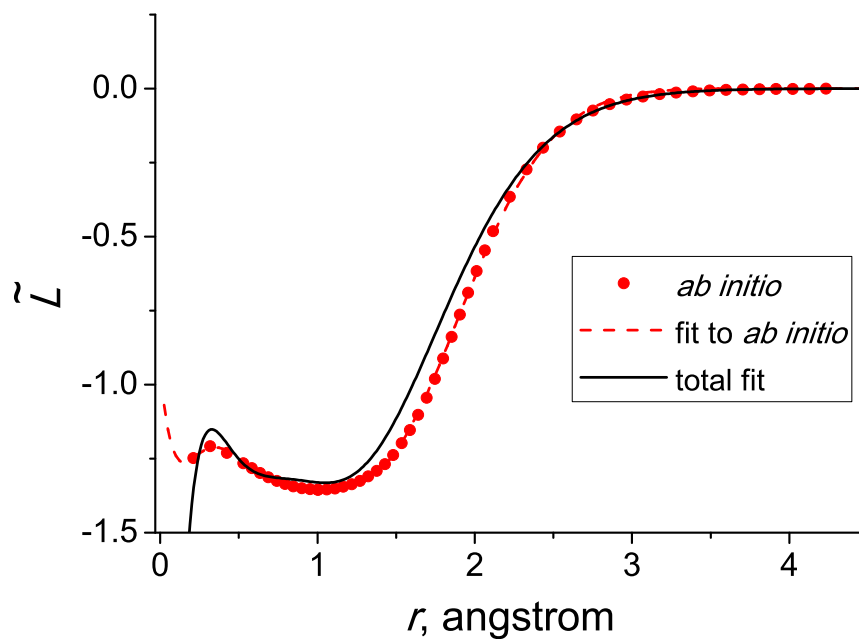

Figure S1: The off-diagonal matrix element of  $L_+$ ,  $\tilde{L}(r) = \langle \Pi | L_+ | \Sigma \rangle$ . The non-monotonic behavior at  $r < 1.5$  Å is a shortcoming of the model.

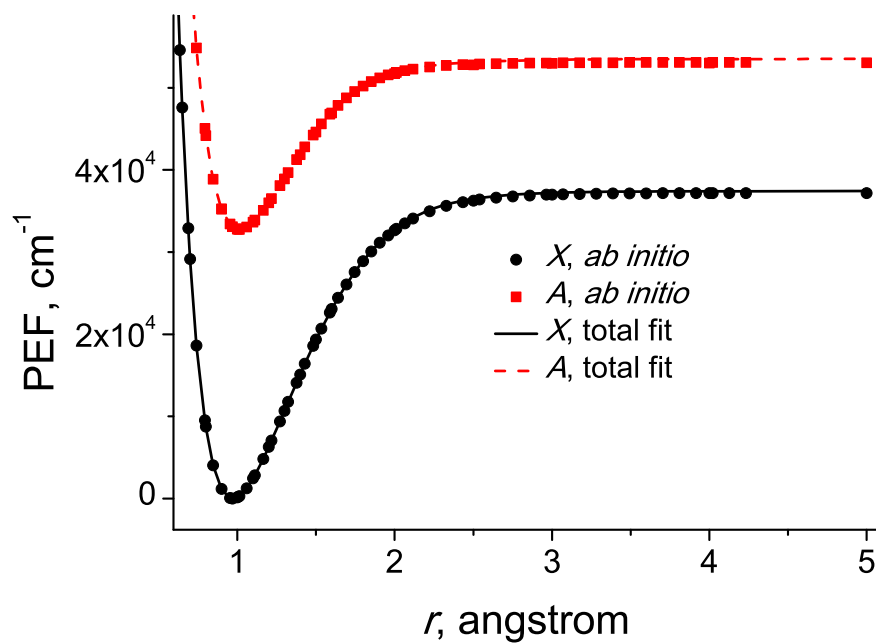

Figure S2: The potential-energy functions of the  $X$  and  $A$  states.

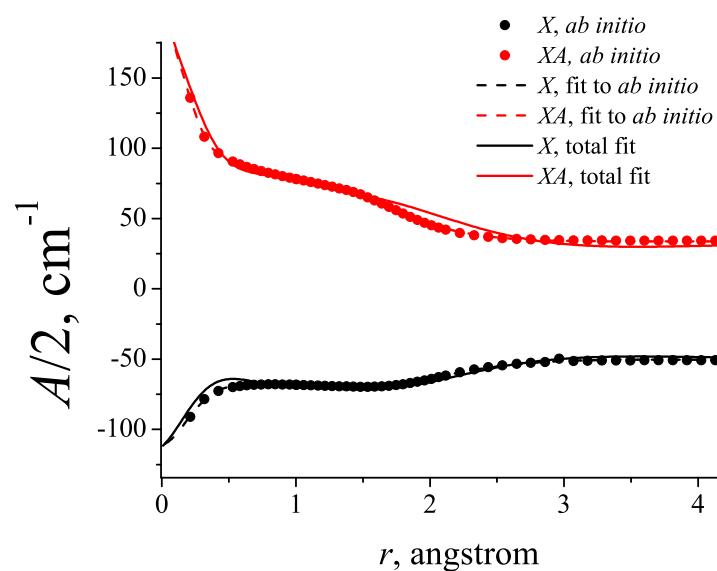

Figure S3: Diagonal,  $A_X$ , and off-diagonal,  $A_{XA}$ , spin-orbit-coupling functions.

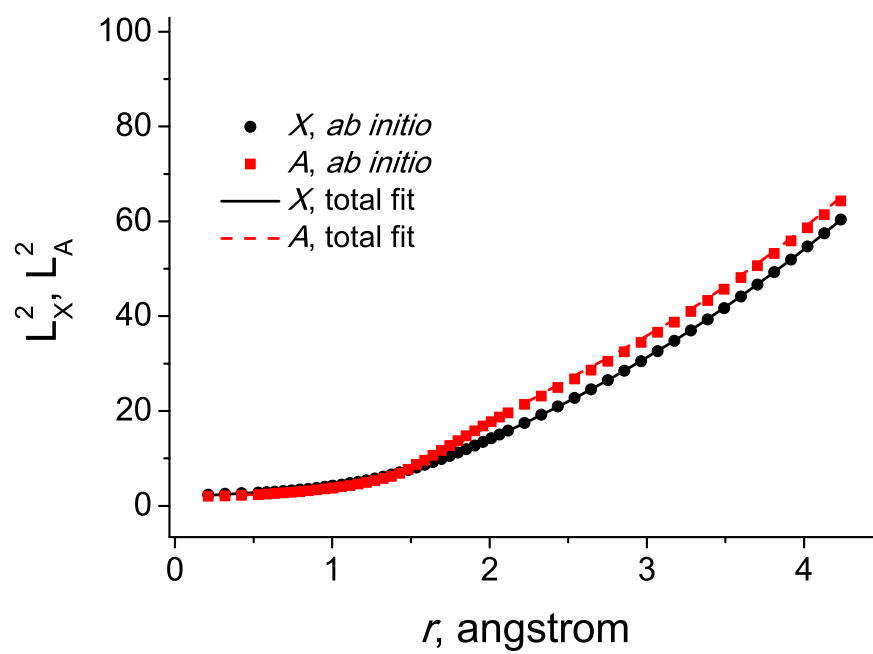

Figure S4: Square of the electronic angular momentum.
